# Supplementary material for: Real-Time Time-Dependent Density Functional Theory Implementation of Electronic Circular Dichroism Applied to Nanoscale Metal-Organic Clusters
Source: arXiv:2007.08560 ancillary file (2020-07-16)
Supplement: Supplementary file 1 [file Supplementary_Information.pdf]

Supplementary Information

# Real-Time Time-Dependent Density Functional Theory Implementation of Electronic Circular Dichroism Applied to Nanoscale Metal-Organic Clusters

Makkonen *et al.*

## Contents

**Supplementary Figures** **2**
S1. Comparison of LR-TDDFT and RT-TDDFT for *R*-methyloxirane . . . 2
S2. Effect of diffuse functions for *R*-methyloxirane . . . 2
S3. Effect of diffuse functions for $G_2-Ag_2^{2+}-G_2$ . . . 3
S4. Effect of diffuse functions for $Ag_{78}$ . . . 3
S5. Convergence of LR-TDDFT calculations with respect to the cut-off energy . . . 4

**Supplementary Tables** **4**
S1. Parameters of diffuse functions . . . 4

**Supplementary Notes** **4**
S1. Convergence of LR-TDDFT calculations with respect to the cut-off energy . . . 4

# Supplementary Figures

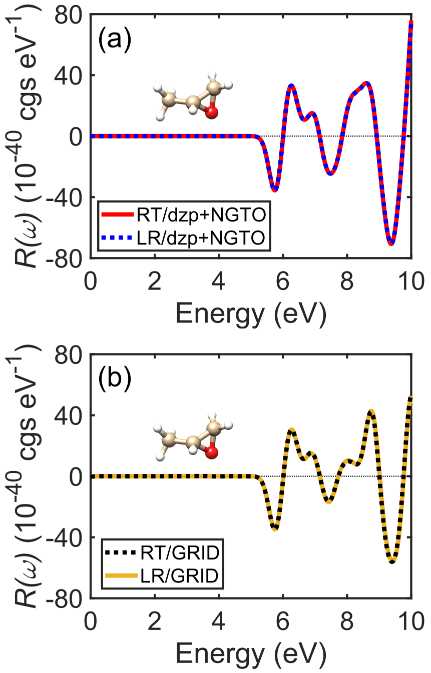


**Supplementary Figure S1: Comparison of LR-TDDFT and RT-TDDFT for $R$-methyloxirane.** Rotatory strength calculated with (a) RT/dzp+NGTO and LR/dzp+NGTO, (b) RT/GRID and LR/GRID. RT and LR results are identical in both LCAO and GRID modes.

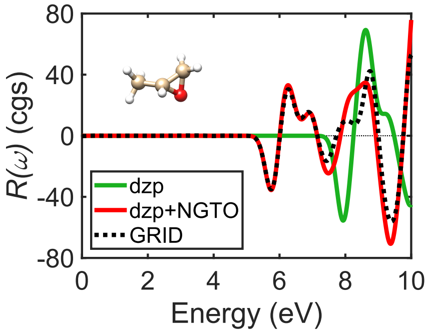


**Supplementary Figure S2: Effect of diffuse functions for $R$-methyloxirane.** Rotatory strength calculated with RT-TDDFT using dzp, dzp+NGTO basis sets (LCAO), and grid mode ($h = 0.2$ Å). The addition of diffuse functions is necessary to capture the two lowest energy peaks that default dzp misses.

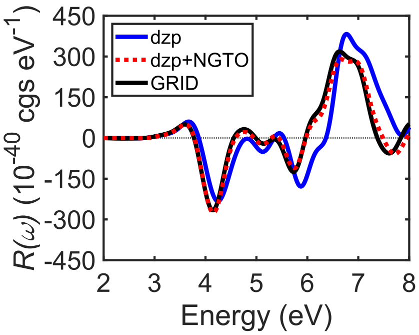


**Supplementary Figure S3: Effect of diffuse functions for $G_2$−$Ag_2^{2+}$−$G_2$.** Rotatory strength calculated with RT-TDDFT using dzp, dzp+NGTO basis sets (LCAO), and grid mode ($h = 0.2$ Å). The dzp+NGTO basis improves the agreement with grid mode.

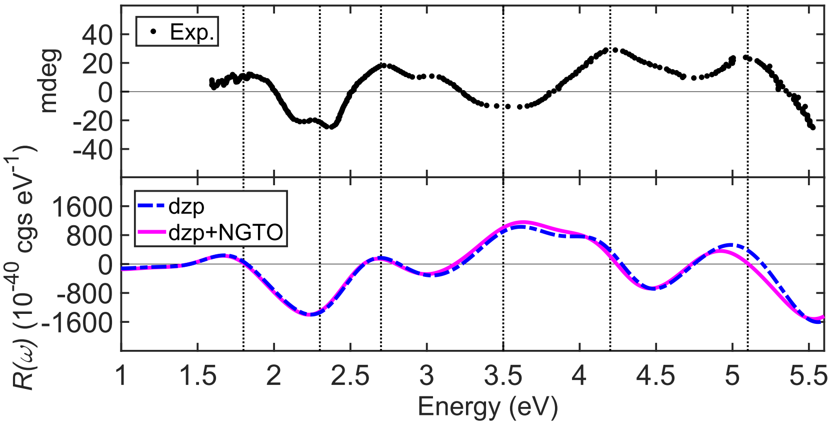


**Supplementary Figure S4: Effect of diffuse functions for $Ag_{78}$.** The experimental (top panel) and calculated (lower panel) ECD spectra. The calculated spectra have been shifted by +0.28 eV. The dzp+NGTO basis doesn't show obvious benefit over dzp.

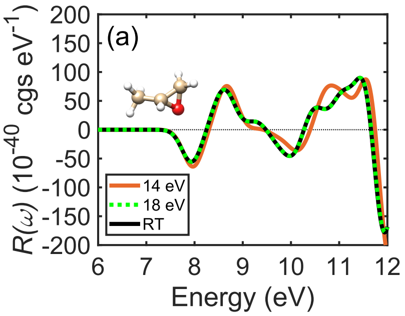


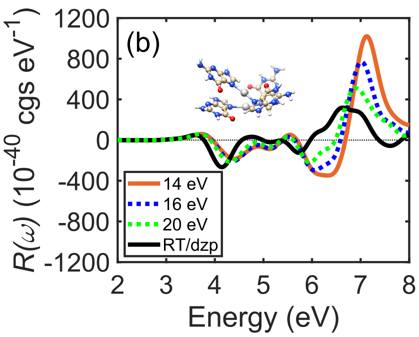


**Supplementary Figure S5: Convergence of LR-TDDFT calculations with respect to the cut-off energy.** Rotatory strength calculated with LR-TDDFT for (a) $R$-methyloxirane (grid mode) and (b) $G_2{-}Ag_2^{2+}{-}G_2$ (LCAO with dzp).

# Supplementary Tables

**Supplementary Table S1: Parameters of diffuse functions.** The Gaussian exponents ($\zeta$-parameters) of the included diffuse functions in dzp+NGTO basis sets from the aug-cc-pvdz basis sets.

| Element | $s$ | $p$ | $d$ |
|---|---|---|---|
| H | 0.02974 | 0.14100 | |
| C | 0.04690 | 0.04041 | 0.15100 |
| N | 0.06124 | 0.05611 | 0.23000 |
| O | 0.07896 | 0.06856 | 0.33200 |
| F | 0.09863 | 0.08502 | 0.46400 |
| P | 0.04170 | 0.03430 | 0.11300 |
| S | 0.05070 | 0.03990 | 0.15200 |

# Supplementary Notes

**Supplementary Note S1: Convergence of LR-TDDFT calculations with respect to the cut-off energy.**

In LR-TDDFT, the Casida equation is typically solved exactly for the complete basis set by iteratively solving their lowest roots. However, in GPAW the LR-TDDFT implementations use a cut-off parameter for the Kohn-Sham transitions, and constructs and diagonalizes the full Casida matrix. The omitted high-energy KS transitions react rapidly to slower excitations in the lower spectral region of interest, i.e., they attempt to screen the excitations as mediated via Hartree-interaction. Thus, the omission of these excitations results in too little screening, which causes blue-shifted excitations with pronounced oscillator strengths as shown in Figure S5. However, typical calculations with LR-TDDFT in GPAW are usually limited to cut-off only to 4-5 eV (common energy range of recorded spectra) due to $O(N^5)$ scaling, which is inadequate according to our findings in the studied cases.
